# Supplementary material for: A Unifying View of Optimism in Episodic Reinforcement Learning
Source: arXiv:2007.01891 source file (2020-07-03)
Supplement: Supplementary file 1 [file appendix_approx_backup.tex]

\section{Results for Linear Function Approximation}\label{app:linproofs}
In this section, we provide proofs of the results in the linear function approximation setting.  
Throughout the analysis, we will use the notation 
\[
C(\delta) = H\sqrt{d \log\pa{\frac{1 + t R^2/\lambda}{\delta}}} + C_P H \sqrt{\lambda d} 
\]
and the definition of the event 
\[
 \mathcal{E}(g,\delta) = \ev{\norm{\pa{M_a - \hM_a}g}_{\Sigma_a} \le C(\delta)}.
\]

We start by proving our key concentration result that will be used for deriving our confidence sets.
\begin{restatable}{proposition}{conc_lin}\label{lem:conc_lin}
Consider the reference model $\wh{P}_a = \Phi \hM_a$ with $\hM_a$ defined in Equation~\eqref{eq:Mhat}.
Then, for any fixed function $g:\Sw\ra [-H,H]$, the following holds with probability at least $1-\delta$:
\[
\norm{\pa{M_a - \hM_a}g}_{\Sigma_a} \le H\sqrt{d \log\pa{\frac{1 + t R^2/\lambda}{\delta}}} + C_P H \sqrt{\lambda d}.
\] 
\end{restatable}
\begin{proof}
We start by rewriting 
\[
 \norm{\pa{M_a - \hM_a}g}_{\Sigma_a} = \norm{\Sigma_a \pa{M_a - \hM_a}g}_{\Sigma_a^{-1}},
\]
and proceed by using the definitions of $\hM_{h,a}$, $\Sigma_{h,a}$ and $W_{h,a}$ as
\begin{align*}
 \Sigma_{h,a} \pa{M_a - \hM_a}g  
 &= \Phi\transpose W_{h,a} \Phi M_a g + \lambda M_a g - 
 \Sigma_{h,a} \Sigma_{h,a}^{-1} \sum_{k=1}^t \II{a_{h,k} = a} \varphi(x_{h,k}) g\pa{x_{h+1,k}}  
\\
&= \Phi\transpose W_{h,a} P_a g - \sum_{k=1}^t \II{a_{h,k} = a} \varphi(x_{h,k}) g\pa{x_{h+1,k}}  + \lambda M_a g 
\\
&=\sum_{k=1}^t \II{a_{h,k} = a} \pa{P_{h}(\cdot|x_{h,k},a_{h,k})g - g(x_{h+1,k})}\varphi\transpose (x_{h,k}) + \lambda M_a g. 
\end{align*}
The first term on the right-hand side is a vector-valued martingale and can be bounded by appealing to 
Theorem~1 of \citet{abbasi2011improved} as
\[
 \norm{\sum_{k=1}^t \II{a_{h,k} = a} \pa{g(x_{h+1,t}) - g\transpose P_{h}(\cdot|x_{h,t},a_{h,t})}\varphi\transpose (x_{h,t})}_{\Sigma_{h,a}^{-1}} 
 \le H\sqrt{d \log\pa{\frac{1 + t R^2/\lambda}{\delta}}}.
\]
The proof is concluded by applying the bound
\[
 \norm{\lambda M_a g}_{\Sigma_{h,a}^{-1}} \le \sqrt{\lambda} \norm{M_a g} \le C_P H \sqrt{\lambda d},
\]
where in the last step we used the assumption that $\onenorm{m_{a}(x)}\le C_P$ and $\infnorm{g}\le H$.
\end{proof}

The following simple result about the sum of inflated exploration bonuses defined in 
Equation~\eqref{eq:expbonus_lin} will also be useful in bounding the regret of the 
two algorithms:
\begin{lemma}\label{eq:sumbound}
For any $h \in [H]$,
 \[
  \sum_a \sum_{t=1}^K \norm{\II{a_{h,t} = a}\varphi(x_{h,t})}_{\Sigma_{h,a,t}^{-1}} \le 2 \sqrt{K A d \log\pa{\frac{1 + K R^2/\lambda}{\delta}}}
 \]
\end{lemma}
\begin{proof}
 The claim is directly proved by the following simple calculations:
 \begin{align*}
 \sum_a \sum_{t=1}^K \norm{\II{a_{h,t} = a}\varphi(x_{h,t})}_{\Sigma_{h,a,t}^{-1}}
 &\le \sqrt{\sum_{a}\sum_{t=1}^K \II{a_{h,t} = a}} \sqrt{\sum_a \sum_{t=1}^K \norm{\II{a_{h,t} = a}\varphi(x_{h,t})}_{\Sigma_{h,a,t}^{-1}}^2}
 \\
 &\le 2 \sqrt{K \sum_a \log\pa{\frac{\textup{det}\pa{\Sigma_{h,a,T}}}{\textup{det}\pa{\lambda I}}}} 
 \le 2 \sqrt{K A d \log\pa{\frac{1 + K R^2/\lambda}{\delta}}},
\end{align*}
where the first inequality is Cauchy--Schwarz and the second follows from Lemma~11 of \citet{abbasi2011improved}.
\end{proof}
Finally, the following result will be useful to bound the scale of the esimated model $\hM_{h,a,t}$ with probability $1$:
\begin{lemma}\label{lem:mhatscale}
 Consider the reference model $\wh{P}_a = \Phi \hM_a$ with $\hM_a$ defined in Equation~\eqref{eq:Mhat}.
Then, for any $C>0$ and any fixed function $g:\Sw\ra [-C,C]$, the following holds with probability $1$:
\[
\norm{\hM_{h,a,t} g} \le \frac{C tR}{\lambda}.
\]
\end{lemma}
\begin{proof}
The statement is proven by straightforward calculations, using the definition of $\hM_{h,a,t}$:
\begin{align*}
 \norm{\hM_{h,a,t} g} &= \norm{\Sigma_{h,a}^{-1} \sum_{k=1}^t \II{a_{h,k} = a} \varphi(x_{h,k}) g\pa{x_{h+1,k}}}
 \\&\le \norm{\Sigma_{h,a}^{-1}}_{\text{op}} \norm{\sum_{k=1}^t \II{a_{h,k} = a} \varphi(x_{h,k}) g\pa{x_{h+1,k}}}
 \le \frac{C}{\lambda} \sum_{k=1}^t \norm{\varphi(x_{h,k})} \le \frac{CtR}{\lambda},
\end{align*}
where the second inequality uses that the operator norm of $\Sigma_{h,a,t}^{-1}$ is at most $\lambda$, and the triangle inequality.
\end{proof}



\subsection{Optimism in state space through local confidence sets}

\subsubsection{Duality Results}
\begin{restatable}{proposition}{dual_approx_1}\label{prop:dual_approx_1}
The optimization problem above is equivalent to solving the optimistic Bellman equations~\eqref{eq:bellman_opt_lin} 
with the exploration bonus defined as
\[
 \CB_{h}(x,a) = D^*\pa{\val^+_{h+1} \middle| \epsilon_h(x,a),\wh{P}_h(\cdot|x,a)}.
\]
\end{restatable}
\begin{proof}%
We first note that, since $\wh{P}_a = \Phi \wh{M}_a$ and using the second constraint, the first 
constraint in the optimization problem can be rewritten as
\[
 \sum_a {\bf q}_{a,h} =\sum_a \wh{M}_a \Phi W_a\Phi\omega_{a,h-1} + \sum_a \pa{\wt{P}_a - \wh{P}_a} 
{\bf q}_{a,h-1}.
\]

Using this, we use a similar argument to Lemma~\ref{lem:duality} to show that strong duality and the KKT conditions hold. We reparameterize by defining $J_h(x,a,x') = q_h(x,a) \wt P_h(x'|x,a)$ and observe that the last constraint in \eqref{eq:primal_lin1} is can be written as $D(J_h(x,a, \cdot) , \wh P_h(\cdot|x,a) \sum_{x'}J_h(x,a,x')) \leq \epsilon_h(x,a) \sum_{x'} J_h(x,a,x')$ which is convex in $J$. It can also be easily observed that the first two constraints, and the objective are linear in $q,J,\omega$. Thus strong duality holds, and the optimal value of the reparameterized optimization problem is equal to the optimal value of the corresponding Lagrangian dual problem. As in the proof of Lemma~\ref{lem:duality}, by using the reverse reparameterization, we can see that the value of the Lagrangian of the modified problem is equal to that of the original problem in \eqref{eq:primal_lin1}. \todoc{Do we need to prove this properly?} Hence, strong duality holds for \eqref{eq:primal_lin1}. It then follows that the KKT conditions also hold for this problem.

Given strong duality, we can find the dual of the problem in \eqref{eq:primal_lin1} by considering the Lagrangian.
The Lagrangian of the optimization problem without the last constraint of the primal can be 
written as
\begin{align}
 \cL(q,\kappa,\omega; \val, \theta) 
 =& \sum_a \iprod{W_a\Phi\omega_a}{r_a + \wh{P}_a 
\val_{h+1} - \Phi \theta_a} \nonumber
\\
&+\sum_{x,a,h} q_h(x,a) \bigg(\pa{\Phi \theta_{h,a}}(x) + \sum_y \kappa(x,a,y) \val_{h+1}(y)  - 
\val_h(x) \bigg) + \val_1(x_1), \label{eq:lag_lin}
\end{align}
for $\kappa(x,a,y) =\wt{P}(y|x,a)-\wh{P}(y|x,a)$. 
Then observe that the optimal value of the primal is equal to 
\[ \min_{\val,\theta}  \max_{q,\omega, \kappa, \wt P \in \cP} \cL(q,\kappa,\omega; \val, \theta).  \]
Observing that $q_h(x,a) \geq 0$ by definition, we can consider the inner maximization over $\wt P_h(\cdot|x,a) \in \cP_h(x,a)$. We get,

\begin{align*}
\max_{ \wt{P}_h(\cdot|x,a) \in \cP_h(x,a)} \sum_y(\wt P_h(y|x,a) - \wh P_h(y|x,a)) \val_{h+1}(y)  = D_*(\val_{h+1} | \wh{P}, \epsilon)
\end{align*}

Substituting this back into \eqref{eq:lag_lin}, we can find the dual from this Lagrangian by observing that the objective function will be given by $\val_1(x_1)$, and using the fact that if $\max_{\omega} \sum_a \iprod{W_a\Phi\omega_a}{r_a + \wh{P}_a \val_{h+1} - \Phi \theta_a} <\infty$, it must be the case that $\iprod{W_a\Phi}{r_a + \wh{P}_a \val_{h+1} - \Phi \theta_a} =0$, and likewise if $\max_{q>0} \sum_{x,a,h} q_h(x,a) (\pa{\Phi \theta_{h,a}}(x) +D_*(\val_{h+1}|\epsilon_{h,a}, \wh P_h(\cdot|x,a))  - \val_h(x)) <\infty$, it must be the case that $\pa{\Phi \theta_{h,a}}(x) +D_*(\val_{h+1}|\epsilon_{h,a}, \wh P_h(\cdot|x,a))  - \val_h(x)\leq 0$.

Thus the dual optimization problem can be written,
\begin{align*}
\underset{\val}{\text{minimize }}  \;& \val_1(x_1) \label{eq:dualtab}
 \\ 
  \text{Subject to } \;& \val_h(x) \geq \pa{\Phi \theta_{h,a}}(x) + D^*\pa{\val_{h+1} \middle| \epsilon_h(x,a),\wh{P}(\cdot|x,a)} \qquad &\forall  (x,a) \in \cZ, h \in [H] \nonumber
   \\& \pa{\Phi W_a \Phi} \theta_{h,a} =   \Phi\transpose W_a\pa{r + \wh{P}\val_{h+1}} \qquad &\forall a \in \cA, h \in [H].  \nonumber
\end{align*}

It is easily seen that the solution to this can be found by solving the optimistic parameteric Bellman equations in \eqref{eq:bellman_lin} via backwards recursion.
\end{proof}




\subsubsection{Regret Bounds}
In this section we prove Theorem~\ref{lem:bonus_lin}.
We first state a result that can be used for constructing confidence intervals around $P(\cdot|x,a)$ in each state-action pair $(x,a)$:
\begin{lemma} \label{lem:conc_lin}
Consider the reference model $\wh{P}_a = \Phi \hM_a$ with $\hM_a$ defined in Equation~\eqref{eq:Mhat}.
Then, for any fixed function $g:\Sw\ra [-H,H]$, the following holds simultaneously for all $(x,a)$ under event $\mathcal{E}(g,\delta)$:
\[
 \pa{P(\cdot|x,a) - \hP(\cdot|x,a)}g \le C(\delta) \norm{\varphi(x)}_{\Sigma_{h,a}^{-1}}.
\]
\end{lemma}
\begin{proof}
The proof is immediate using the definition of the event $\mathcal{E}(g,\delta)$ and the Cauchy--Schwarz inequality:
 \begin{align*}
  \pa{P(\cdot|x,a) - \hP(\cdot|x,a)}g &= \biprod{\varphi(x)}{\bpa{M_a - \hM_a} g}
  \le \norm{\varphi(x)}_{\Sigma_{h,a}^{-1}} \norm{\pa{M_a - \hM_a} g}_{\Sigma_{h,a}}.
 \end{align*}
\end{proof}
In order to show that the confidence set defined in Equation~\eqref{eq:CBonus_lin} includes the true transition model, we need to 
show that the above bound holds uniformly for all value functions in stage $h+1$ that can be ever produced by solving the optimistic
Bellman equations~\eqref{eq:bellman_opt_lin}. 
We observe that, with exploration bonuses of the form $\CB_{h,t}(x,a) = \alpha \norm{\phi(x)}_{\Sigma_{t,a,h}^{-1}}$,
these functions take the form 
\[
 V^+_{t,h}(x) = \min\ev{H-h,\,\max\ev{\iprod{\varphi(x)}{\theta_{t,a,h}} + \alpha\norm{\phi(x)}_{\Sigma_{t,a,h}^{-1}}}},
\]
which is a smoothly parametrized function of the feature vector $\varphi(x)$. Let $\V_{h+1,t}$ denote the set of such functions in any stage $h+1$ and episode $t$.

For our results, it will be necessary to bound the covering number of this class of functions. This is done in the following Lemma, whose proof is similar to that of Lemma D.6 of \cite{jin2020provably}.
\begin{lemma} \label{lem:cover}
Let $\cN(\V,\varepsilon)$ be the $\varepsilon$-covering number of some set $\V$ with respect to the distance $\|V-V'\|_\infty = \sup_{x \in \cS} |V(x) - V'(x)|$. Then, for any stage $h=1,\dots, H$ and episode $t$,
\[ \log(\cN(\V_{h+1,t}, \varepsilon)) \leq Ad \log(1+4BR/\varepsilon) + d^2A \log(1+4RC(d)/(\lambda \varepsilon^2)) \]
where $R$ is such that $\|\varphi(x)\|_2 \leq R \, \forall x \in \cS$, $\lambda$ is such that the minimum eigenvalue, $\lambda_{\min}(\Sigma_{h,a})\geq \lambda \, \forall a \in \cA, h\in [H]$.
\todoc{check norm, define bound $B$}
\end{lemma}
\begin{proof}
The proof is similar to that of  Lemma D.6 of \cite{jin2020provably}. For ease of notation, we drop dependence on $t$ and,  for a fixed $C(d)$, define the sets 
\begin{align*}
 \V_h = \bigg\{ V_h:\cS \to [0,H-h+1] : &\forall a \in \cA \, \exists \theta_{h,a} \in \bR^d \|\theta_{h,a} \|\leq B, \Sigma_{h,a} \in \bR^{d \times d} , \lambda_{\min}(\Sigma_{h,a}) \geq \lambda \text{ s.t. }
 \\ & V_h(x) = \min\{ H-h+1, \max_{a \in \cA}\{ \varphi(x)\transpose \theta_{h,a} + C(d) \| \varphi(x)\|_{\Sigma^{-1}_{h,a}} \} \} \bigg\} 
 \end{align*}

 
For any $h\in [H]$, let $V_h,\wt V_h \in \V_h$ so $V_h(x) = \min\{ H-h+1, \max_{a \in \cA}\{ \varphi(x)\transpose \theta_{h,a} + C(d) \| \varphi(x)\|_{\Sigma^{-1}_{h,a}} \} \} \bigg\} $ and $\wt V_h(x) = \min\{ H-h+1, \max_{a \in \cA}\{ \varphi(x)\transpose \wt \theta_{h,a} + C(d) \| \varphi(x)\|_{\wt \Sigma^{-1}_{h,a}} \} \} \bigg\} $ . Then,
\begin{align*}
\|V_h - \wt V_h\|_\infty &= \sup_{x \in \cS} \bigg|  \min\{ H-h+1, \max_{a \in \cA}\{ \varphi(x)\transpose \theta_{h,a} + C(d) \| \varphi(x)\|_{\Sigma^{-1}_{h,a}} \} \}  
	\\ & \hspace{30pt} -  \min\{ H-h+1, \max_{a \in \cA}\{ \varphi(x)\transpose \wt \theta_{h,a} + C(d) \| \varphi(x)\|_{\wt \Sigma^{-1}_{h,a}} \} \}  \bigg |
\\ & \leq \sup_{x \in \cS} \bigg|\max_{a \in \cA}\{ \varphi(x)\transpose \theta_{h,a} + C(d) \| \varphi(x)\|_{\Sigma^{-1}_{h,a}} \}  - \max_{a \in \cA}\{ \varphi(x)\transpose \wt \theta_{h,a} + C(d) \| \varphi(x)\|_{\wt \Sigma^{-1}_{h,a}} \} \bigg |
\\ & \leq \sup_{x \in \cS, a \in \cA} \bigg| \varphi(x)\transpose \theta_{h,a} + C(d) \| \varphi(x)\|_{\Sigma^{-1}_{h,a}}  - \varphi(x)\transpose \wt \theta_{h,a} + C(d) \| \varphi(x)\|_{\wt \Sigma^{-1}_{h,a}}  \bigg| 
\\ & \leq \sup_{x \in \cS,a \in \cA} \bigg| \varphi(x)\transpose (\theta_{h,a} - \wt \theta_{h,a})  + \sqrt{ \varphi(x) \transpose (C(d) \Sigma_{h,a}^{-1} - C(d) \wt \Sigma_{h,a}^{-1}) \varphi(x)} \bigg|
\\ & \leq \sup_{a \in \cA} R\| \theta_{h,a} - \wt \theta_{h,a}\|_2 + \sup_{a \in \cA} R\|C(d) \Sigma_{h,a}^{-1} - C(d) \wt \Sigma_{h,a}^{-1} \|
\\ & \leq  \sup_{a \in \cA} R \| \theta_{h,a} - \wt \theta_{h,a}\|_2 + \sup_{a \in \cA} R C(d)\| \Sigma_{h,a}^{-1} - \wt \Sigma_{h,a}^{-1} \|_F
\end{align*}
since $\|\varphi(x)\|_2 \leq  R$  and we have used $\|A\|$ to denote the matrix operator norm and $\|A\|_F$ the Frobenius norm of a matrix $A$.

We then note that the $\varepsilon/2$-covering number of the set $\Theta = \{ (\theta_a)_{a \in \cA}: \theta_a \in \bR^d, \, \sup_{a \in \cA}\|\theta_a\|_2 \leq B \}$ is bounded by $(1+4B/\varepsilon)^{Ad}$, and that $\varepsilon/2$-covering number of the set $\Gamma = \{  (\Sigma_a)_{a \in \cA}: \Sigma_a \in \bR^{d\times d}, \,\sup_{a \in \cA} \|\Sigma_a\|_F \leq 1/\lambda \}$ is bounded by $(1+4/(\lambda \varepsilon^2))^{d^2A}$. These results follow due to the standard fact that the $\varepsilon$-covering number of a ball in $\bR^d$ with radius $R>0$ with $\ell_2$ distance is bounded by $(1+2R/\varepsilon)^d$, and that $\Theta$ is $(dA)$-dimensional, while $\Gamma$ can be viewed as being $(d^2A)$-dimensional.

From the above discussion, we can conclude that for any $V_h \in \V_h$, there is a $\wt V_h$ parameterized by $\wt \theta_h$ in the $\varepsilon/2$-covering of $\Theta_h$, and $\Sigma_h$ in the $\varepsilon/2$-covering of $\Gamma_h$ such that,
\[ \|V_h - \wt V_h\|_\infty \leq R \varepsilon/2 + RC(d) \varepsilon/2. \]
By rescaling of the covering numbers \todoc{add reference or explanation}, we can see that the logarithm of the $\varepsilon$-covering number of $\V_h$ can be bounded by
\begin{align*}
\log(\cN(\V_h,\varepsilon)) &\leq \log(\cN(\Theta_h, \varepsilon/(2R))) + \log(\cN(\Gamma_h, \varepsilon/(2C(d)R)) 
\\ &\leq Ad \log(1+4BR/\varepsilon) + d^2A \log(1+4RC(d)/(\lambda \varepsilon^2))
\end{align*}
giving the result.

\todoc{Check why $\Sigma$ case has $\varepsilon^2$}
\end{proof}


\todoc{I don't follow why this is here?: Supposing that the covering number of this class is $\mathcal{N}$, 
we can define the event 
\[
\mathcal{F}(\delta) = \ev{\sup_{g\in\V_{h+1}} \norm{\pa{M_a - \hM_a}g}_{\Sigma_a} \le C(\delta/\mathcal{N})}.
\]
The following statement bounds the probability of this event:
}
\begin{lemma}
Consider the reference model $\wh{P}_a = \Phi \hM_a$ with $\hM_a$ defined in Equation~\eqref{eq:Mhat}.
Then, the following holds with probability at least $1-\delta$:
\[
 \pa{P_h(\cdot|x,a) - \hP_{h,t}(\cdot|x,a)} \val_{h+1,t} \le C(\delta/\mathcal{N}) \norm{\varphi(x)}_{\Sigma_{h,a}^{-1}}.
\] 
\end{lemma}
\begin{proof}
The result follows by combining Lemmas~\ref{lem:conc_lin}~and~\ref{lem:cover}. In particular for any $\val_{h+1,t} \in \V_{h+1,t}$, it follows that there exists a $\wt V_{h+1,t}$ in the $\varepsilon$-cover of $\V_{h+1,t}$ such that $\|V_{h+1,t} - \wt V_{h+1,t}\|_\infty \leq \varepsilon$. Consequently,
\begin{align*}
&\pa{P_h(\cdot|x,a) - \hP_{h,t}(\cdot|x,a)} \val_{h+1,t} = \pa{P_h(\cdot|x,a) - \hP_{h,t}(\cdot|x,a)} \wt V_{h+1,t}
	\\ & \hspace{150pt} + \pa{P_h(\cdot|x,a) - \hP_{h,t}(\cdot|x,a)}(\val_{h+1,t} -\wt V_{h+1,t}) 
\\ &\leq \pa{P_h(\cdot|x,a) - \hP_{h,t}(\cdot|x,a)} \wt V_{h+1,t} + \|\varphi(x)\|_{\Sigma_{h,a,t}^{-1}} \| (M_{h,a}-\wh M_{h,a,t})(\val_{h+1,t} -\wt V_{h+1,t}) \|_{\Sigma_{h,a,t}} 
\\ & \leq  \pa{P_h(\cdot|x,a) - \hP_{h,t}(\cdot|x,a)} \wt V_{h+1,t} +  \|\varphi(x)\|_{\Sigma_{h,a,t}^{-1}} \| \Sigma_{h,a,t}M_{h,a} - \sum_{s=1}^t \varphi(x_{h,s})\be_s \|_{\Sigma_{h,a,t}^{-1}}
\\ & \leq \pa{P_h(\cdot|x,a) - \hP_{h,t}(\cdot|x,a)} \wt V_{h+1,t} + \lambda \|\varphi(x)\|_{\Sigma_{h,a,t}^{-1}} 	\bigg \|(M_{h,a}-  \sum_{s=1}^t \varphi(x_{h,s})\be_s)(\val_{h+1,t} - \wt V_{h+1,t}) \bigg \|_{\Sigma_{h,a,t}^{-1}}
	\\ &\hspace{70pt} +  \|\varphi(x)\|_{\Sigma_{h,a,t}^{-1}} \bigg \| \bigg(\sum_{s=1}^t \varphi(x_{h,s}) \varphi(x_{h,s}) \transpose M_{h,a} - \sum_{s=1}^t \varphi(x_{h,s})\be_s \bigg) (\val_{h+1,t} - \wt V_{h+1,t}) \bigg \|_{\Sigma_{h,a,t}^{-1}} 
\\ & \leq  \pa{P_h(\cdot|x,a) - \hP_{h,t}(\cdot|x,a)} \wt V_{h+1,t} + \lambda ^{1/2}\|\varphi(x)\|_{\Sigma_{h,a,t}^{-1}} (d+tR)\varepsilon
	\\ & \hspace{70pt} +  \|\varphi(x)\|_{\Sigma_{h,a,t}^{-1}} \lambda^{-1/2} \sum_{s=1}^t \|\varphi(x_{h,s})\|_2 \| (\varphi(x_{h,s})\transpose M_{h,a} - \be_s) (\val_{h+1,t} - \wt V_{h+1,t})\|_2 
\\ & \leq  \pa{P_h(\cdot|x,a) - \hP_{h,t}(\cdot|x,a)} \wt V_{h+1,t} +  \|\varphi(x)\|_{\Sigma_{h,a,t}^{-1}}  \lambda^{-1/2} tR\varepsilon + \lambda^{1/2} \|\varphi(x)\|_{\Sigma_{h,a,t}^{-1}} (d+tR)\varepsilon
\end{align*}

\todoc{check lower order term do we need $\lambda >1$?
}
To bound the first term, we use a union bound over all $\wt V_{h+1,t}$ in the $\varepsilon$-covering of $\V_{h+1,t}$ and Theorem~\ref{thm:cb_lin} to see that for any $\wt V_{h+1,t}$ in the $\varepsilon$-covering, with probability greater than $1-\delta$,
\begin{align*}
&\pa{P_h(\cdot|x,a) - \hP_{h,t}(\cdot|x,a)} \wt V_{h+1,t} \leq  \sqrt{C(\delta) + \log(\cN(\V_{h+1,t},\varepsilon)/\delta)}  \|\varphi(x)\|_{\Sigma_{h,a,t}^{-1}}
\\ & \leq  \sqrt{C(\delta) + \log(1/\delta) + Ad \log(1+4BR/\varepsilon) + d^2A \log(1+4RC(d)/(\lambda \varepsilon^2))}  \|\varphi(x)\|_{\Sigma_{h,a,t}^{-1}}
\end{align*}
\todoc{sort out constants}

Setting $\varepsilon = \lambda^{1/2}/( tR)$ gives the result. \todoc{add choice of $C$ to statement}

\todoc{did not use this: will also need bounding the Lipschitz constants?}
\end{proof}


Thus, setting the width of the confidence interval in stage $h$ of episode $t$ as
\[
 \alpha_{h,t} = C_{t}(\delta/\mathcal{N}) = H\sqrt{d \log\pa{\frac{1 + t R^2/\lambda}{\delta}} + 2d^2 A \log(5RC(d) t^2R^2) + 2AD \log(5BR^2t)} + C_P H \sqrt{\lambda d}
\]
shows that $P\in\cP$ indeed holds with probability at least $1-\delta$.
\todoc{check constants and lower order terms}

In this setting, we can use the results of Theorem~\ref{thm:reggen} to bound the regret of this algorithm in terms of the sum of the confidence bounds. This gives the following result,
\begin{theorem}
With probability greater than $1-\delta$, the regret of the algorithm solving the optimistic parametric Bellman equations in \eqref{eq:opb} in each episode with $\CB_{h,t}(x,a) = \|\varphi(x)\|_{\Sigma_{h,a,t}^{-1}} \alpha_{h,t}$ incurs regret,
\[ \Reg_T \leq \]
so we can conclude that the regret is $\wt O (\sqrt{H^3d^3 AT})$. 
\end{theorem}
\begin{proof}
We first note by definition of $D$ in this case, it holds that $D_*(-\val^+_{h+1,t}|\epsilon_{h,t}(x,a), \wh{P}_{h,t}) \leq \epsilon_{h,t}(x,a)$ and $D_*(\val^+_{h+1,t}|\epsilon_{h,t}(x,a), \wh{P}_{h,t}) \leq \epsilon_{h,t}(x,a)$ \todoc{add proof/justification}
We use Theorem~\ref{thn:reggen} to see that the regret can be bounded by,
\begin{align*}
\Reg_T &\leq \sum_{t=1}^K \sum_{h=1}^H \bigg( D_*(-\val^+_{h+1,t}|\epsilon_{h,t}(x_{h,t},a_{h,t}), \wh{P}_{h,t}) +  D_*(\val^+_{h+1,t}|\epsilon_{h,t}(x_{h,t},a_{h,t}), \wh{P}_{h,t})  + H \sqrt{2T \log(1/\delta)} 
\\ & \leq \sum_{t=1}^K \sum_{h=1}^H 2\alpha_{h,t} \|\varphi(x_{h,t}) \|_{\Sigma_{h,a_{h,t},t}^{-1}} + H \sqrt{2T \log(1/\delta)} \tag*{(By definition of $D_*$)}
\\ & \leq C_{K}(\delta/\cN) \sum_{t=1}^K \sum_{h=1}^H  \|\varphi(x_{h,t}) \|_{\Sigma_{h,a_{h,t},t}^{-1}} + H \sqrt{2T \log(1/\delta)} \tag*{(Since $C_{t}(\delta/\cN)$ is increasing in $t$)}
\\ & \leq C_{h,K}(\delta/\cN) 2H \sqrt{KAd \log(\frac{1+KR^2/\lambda}{\delta})} \tag*{(By Lemma~\ref{eq:sumbound})}
\end{align*}
The result then follows by the definition of $C_t(\delta/\cN)$ and noting that $C_t(\delta/\cN) = \wt O(Hd \sqrt{A})$.
\end{proof}

\if0
Thus, appealing to Theorem~\ref{thm:reglin} \todoc{do we need a general result for the regret of an algorithm in the linear setting? Or can we use the standard ones?} and Lemma~\ref{lem:sumbound}, we can show that the regret of the algorithm is bounded by
 \begin{align*}
  \Reg_T  &\le \sum_{h=1}^H \sum_a \sum_{t=1}^K \alpha_{h,t} \norm{\II{a_{h,t} = a}\varphi(x_{h,t})}_{\Sigma_{h,a,t}^{-1}} 
  \\
  &\le 
  H^2 d\sqrt{KA} \log\pa{\frac{1 + t R^2/\lambda}{\delta}} + H^2 \sqrt{d KA \log\pa{\frac{1 + t R^2/\lambda}{\delta}} \log \mathcal{N}} + C_P H \sqrt{\lambda d \log\frac{1 + t R^2/\lambda}{\delta}}.
 \end{align*}
Showing that $\log \mathcal{N} = \wt{O}(d^2)$ shows that the regret is of order $H^2 \sqrt{d^3 KA} = \sqrt{H^3 d^3 TA}$.
\fi

\if0
\redd{\textbf{Older stuff:}
\begin{restatable}{lemma}{lem:bonus_lin}\label{lem:bonus_lin}
 The confidence set defined in Equation~\eqref{eq:CBonus_lin} includes the true transition model $P(\cdot|x,a)$ with the choice
 \[
 \epsilon_h(x,a) =  2H \norm{\varphi(x)}_{\Sigma_{h,a}^{-1}} \sqrt{d \log \bigg(1+ \frac{t}{d} \bigg)  + \log\pa{\frac{1}{\delta}} + \log \mathcal{N}(\F,d_\varphi,...) }
\]
simultaneously for all $(x,a)$ with probability greater than $1-\delta$.
\todoG{Replace the covering number by its actual value...?}
\end{restatable}
Setting $\lambda = 1$ gives, $|(\wh{P} - P)g| \leq 2H \|\varphi(x)\|_{\lambda_a^{-1/2}} \sqrt{d \log \bigg(1+ \frac{t}{d} \bigg)  - \log(\delta)}$ with probability greater than $1-\delta$ for any fixed $g \in \cC(\cF_{L,H}, \epsilon)$. Therefore, with probability greater than $1-\delta\cN(\cF_{L,H}, \epsilon)$ it must hold for all $g \in \cC(\cF_{L,H}, \epsilon)$ where $\cN(\cF_{L,H}, \epsilon)$ is the $\epsilon$ covering number. \todoc{specify norm}. We note that since $\cF_{L,H}$ is the set of all bounded lipschitz functions of $\varphi(x) \in \bR^d$ and $\|\varphi(x)\|\leq 1$ \todoc{do we make this constraint on the norm? do we need it?}, it follows from standard results that $\cN(\cF_{L,H}, \epsilon) \leq $}
\fi


\subsection{Optimism in feature space through global constraints}
\subsubsection{Proof of Theorem~\ref{thm:regret_lin_global}}
We start by observing that the exploration bonuses in this case have the simpler form
$\CB_{h,t}(x,a) = \iprod{\varphi(x)}{B_{t,a,h}}$, which implies that the value functions
the form 
\[
 V^+_{t,h}(x) = \min\ev{H-h,\,\max\ev{\iprod{\varphi(x)}{\theta_{t,a,h}} + \alpha\norm{\phi(x)}_{\Sigma_{t,a,h}^{-1}}}},
\]
which is a smoothly parametrized function of the feature vector $\varphi(x)$. Supposing that the covering number of this class is $\mathcal{N}$, 
we can define the event 
\[
\mathcal{F}(\delta) = \ev{\sup_{g\in\V_{h+1}} \norm{\pa{M_a - \hM_a}g}_{\Sigma_a} \le C(\delta/\mathcal{N})}.
\]
The following statement bounds the probability of this event:
\begin{lemma}
Consider the reference model $\wh{P}_a = \Phi \hM_a$ with $\hM_a$ defined in Equation~\eqref{eq:Mhat}.
Then, the following holds with probability at least $1-\delta$:
\[
 \pa{P(\cdot|x,a) - \hP(\cdot|x,a)}g \le C(\delta/\mathcal{N}) \norm{\varphi(x)}_{\Sigma_{h,a}^{-1}}.
\] 
\end{lemma}




For each individual stage $h$, the sum of the confidence bonuses can be bounded as follows:
\begin{align*}
 \sum_{t=1}^K \textup{CB}_{h,t}^\dag(x_{h,t},a_{h,t}) &= \sum_{t=1}^K \sum_{a} \II{a_{h,t} = a} \iprod{\varphi(x_{h,t})}{B_{h,a,t}}
 \\
 &\le \sum_a \sum_{t=1}^K \norm{\II{a_{h,t} = a}\varphi(x_{h,t})}_{\Sigma_{h,a,t}^{-1}}\norm{B_{h,a,t}}_{\Sigma_{h,a,t}}
 \\
 &\le \epsilon \sqrt{\sum_{a}\sum_{t=1}^K \II{a_{h,t} = a}} \sqrt{\sum_a \sum_{t=1}^K \norm{\II{a_{h,t} = a}\varphi(x_{h,t})}_{\Sigma_{h,a,t}^{-1}}^2}
 \\
 &\le 2 \epsilon \sqrt{K \sum_a \log\pa{\frac{\textup{det}\pa{\Sigma_{h,a,T}}}{\textup{det}\pa{\lambda I}}}} \le 2 \epsilon \sqrt{K A d \log\pa{\frac{1 + t R^2/\lambda}{\delta}}},
\end{align*}
where we used our bound on $B$ and a standard argument to bound the self-normalized sum in the last step.





\subsection{Regret Bounds}
